# Supplementary material for: Wiggins: Detecting Valuable Information in Dynamic Networks Using Limited Resources
Source: arXiv:1504.03275 source file (2015-07-29)
Supplement: Supplementary file 1 [file appendix.tex]

\section{Proof of Lemma 1}\label{app:proof}

 Let $i=i_{t, S}$ be an item. The probability that $i$ is still uncaught at time $t'$ is $(1-\p(S))^{c(t'-t)}$, and its freshness at $t'$ is $\theta^{t' - t}$. Therefore, $i$ imposes the load $\theta^{t'-t}$ to the system at time $t'$, with probability $(1-\p(S))^{c(t'-t)}$, and zero otherwise. Since the probability of $i_{t,S}$ being generated is $\pi(S)$ we have
\begin{align*}
 \cost{\p} &= \limsup_{t\rightarrow\infty}\frac{1}{t}\sum_{t'=0}^t\E(L_{\sys}(t')) = \limsup_{t\rightarrow \infty} \E\paran{L_{\sys}(t)} \\
 &=\lim_{t\rightarrow \infty} \sum_{S\in \F} \pi(S) \paran{1 + \theta\cdot(1-\p(S))^c + \ldots + \theta^t\cdot(1-\p(S))^{ct}} \\ 
 &=
 \sum_{S\in \F} \frac{\pi(S)}{1-\theta(1-\p(S))^c},
\end{align*}
\ahmad{where we used the fact that for any convergent sequence $\set{a_i}_{i\in\mathbb{N}}$ we have $\lim\limits_{t\rightarrow\infty}\frac{\sum_{i=1}^t a_i}{t} = \lim\limits_{i\rightarrow\infty}a_i$.}\qed
